# Supplementary material for: Stabilizability of Vector Systems with Uniform Actuation Unpredictability
Source: arXiv:2105.04652 source file (2021-05-17)
Supplement: Supplementary file 1 [file 10_appendix_link.tex]

\section{Appendices}
\label{sec: Appendix Link}

Please see \href{https://drive.google.com/drive/folders/15UNnTkRN8-IHNqA4ClYSzgkfd3HP39kW?usp=sharing}{here} for a version of the paper with appendices (\url{https://drive.google.com/drive/folders/15UNnTkRN8-IHNqA4ClYSzgkfd3HP39kW?usp=sharing}).
